# Supplementary material for: Optimizing the Consumption of Spiking Neural Networks with Activity Regularization
Source: arXiv:2204.01460 source file (2022-04-04)
Supplement: Supplementary file 1 [file Supplementary.tex]

\section{Supplementary Material}
\subsection{Experiments on CIFAR-10}

\subsubsection{Multi-layer perceptron}
We run the same experiment on CIFAR-10. The MLP is transformed to a 3072-300-100-10 architecture. The training, calibration and inference procedures are kept the same. As the dataset is more complicated, we allow the precision to have a difference of $1.5\%$ with respect to the baseline performance. Table \ref{tab:results_cifar10_mlp} and Fig. \ref{fig:curves_cifar10_mlp} summarize the results on a few regularizers. We observe that the SynOps are reduced by more than $11\times$ in the MLP with $L_{0.5}$ regularizer, and that the precision of the SNN is increased with respect to the baseline.

\begin{table}[h!]
\centering
\resizebox{1.0\linewidth}{!}{\begin{tabular}{lrrrrrrr}
& \textbf{Spikes}  & \textbf{EFLOPS} & \textbf{SynOps} & \textbf{Accuracy} \\ 
& & & & (DNN/SNN) \\
\hlineB{3}
MLP Baseline & 54435 & 937268 & 3329247 & 50.78\% / 49.41\%\\
\hline
\textbf{Reg. @ $\lambda_{reg}$}  & \textbf{$\Delta$Spikes}  & \textbf{$\Delta$EFLOPS} & \textbf{$\Delta$SynOps} & \textbf{$\Delta$Accuracy} \\
%\hline
%MLP Baseline & 54435 & 937268 & 3329247 & 50.78\% / 49.41\%\\
\hline
L2@0.01  & 2.73x & 1.01x & 7.74x & 2.34\% / 1.37\% \\
L1@0.007 & 4.35x & 1.01x & 10.90x & 2.93\% / 0.20\% \\
L0.5@0.005 & \textbf{5.87x} & 1.01x & \textbf{11.37x} & -0.78\% / 0.98\% \\

\hlineB{3}

\end{tabular}}
\caption{Regularization results for MLP.} 
\label{tab:results_cifar10_mlp}
\end{table}

\begin{figure}[h!]
    \centering
    {{\includegraphics[width=8.5cm]{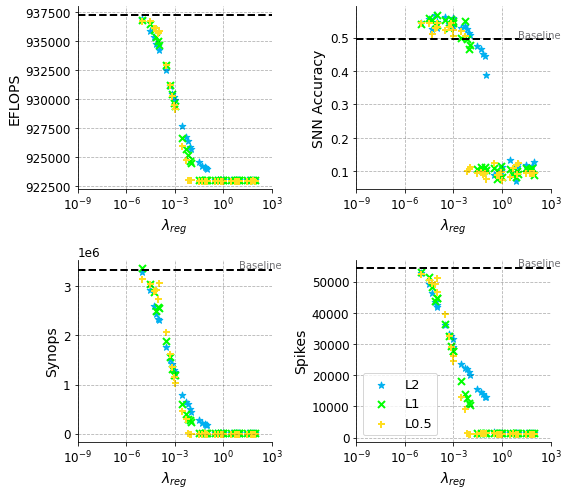}}}%
    \caption{Metrics relative to the regularization constant $\lambda_{reg}$ in the converted SNN MLP architecture for CIFAR-10 dataset.} %
    \label{fig:curves_cifar10_mlp}%
\end{figure}
%% TODO

\subsubsection{LeNet-5}

LeNet-5 architecture was adapted by removing the zero-padding layer on the input to support CIFAR-10 images. When converting this network to SNN using the standard procedure, the baseline model resulted in bad accuracy. We. therefore increased the number of steps to evaluate the SNN from $50$ as $100$. However, it can be observed from Fig. \ref{fig:curves_cifar10_lenet} that the conversion impacts the performance of the baseline model (28\% of accuracy drop). 
The baseline is chosen to be the model with the most number of spikes emitted (LeNet-5, $L_2$ @ $1e-5$), egularized network lays in this accuracy region, and allow a maximum difference in accuracy of 1.5\% after conversion.
The result of this experience are summarized in Table \ref{tab:results_cifar10_lenet}, and we report the performance of the model without regularization for completeness. It shows that SynOps can still be reduced up to $4.91\times$ using activity regularization without impacting the accuracy too much. 

This can be in part explained by the complexity of the CIFAR-10 dataset, which is less sparsifiable than MNIST. Here, $L_1$ performs better than the other regularizers, suggesting that $L_{0.5}$ may be too aggressive for CNN architecture. As the model contains less parameters, the information has less opportunity to be combined with information coming from other parts of the input image. 

\begin{table}[h!]
\centering
\resizebox{1.0\linewidth}{!}{\begin{tabular}{lrrrrrrr}
& \textbf{Spikes} & \textbf{EFLOPS} & \textbf{SynOps} & \textbf{Accuracy} \\ 
& & & & (DNN/SNN) \\
\hlineB{3}
LeNet-5 w/o regularizer & 5896027 & 610225 & 338563031 & 61.72\% / 43.75\%\\
L2 @ 1e-05 (Baseline) & 7105009 & 603957 & 436288873 & 64.06\% / 65.62\%  \\
\hline
\textbf{Reg. @ $\lambda_{reg}$}  & \textbf{$\Delta$Spikes}  & \textbf{$\Delta$EFLOPS} & \textbf{$\Delta$SynOps} & \textbf{$\Delta$Accuracy} \\
\hline
L2 @ 0.01  & 3.06x & 1.12x & 3.97x & 2.54\% / 0.20\% \\
L1 @ 0.001  & \textbf{3.84x} & 1.17x & \textbf{4.91x} & 1.76\% / -0.78\% \\
L0.5 @ 5e-05  & 1.50x & 1.03x & 1.54x & 2.54\% / -0.98\% \\
\hlineB{3}

\end{tabular}}
\caption{Regularization results for LeNet-5.} 
\label{tab:results_cifar10_lenet}
\end{table}

\begin{figure}[h!]
    \centering
    {{\includegraphics[width=8.5cm]{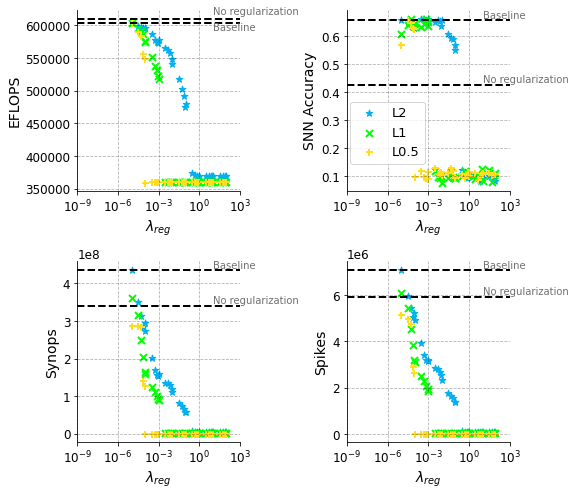}}}%
    \caption{Metrics relative to the regularization constant $\lambda_{reg}$ in the converted SNN MLP architecture for CIFAR-10 dataset.} %
    \label{fig:curves_cifar10_lenet}%
\end{figure}
